# Supplementary material for: Deep Bilateral Learning for Real-Time Image Enhancement
Source: arXiv:1707.02880 source file (2017-08-22)
Supplement: Supplementary file 1 [file appendix.tex]

\section{Appendix}
% \subsection{Slicing gradient}
% \label{sec:slicing_gradient}
%
% We give here the analytical sub-derivatives necessary to backpropagate through
% the slicing layer presented in Section~\ref{sec:trainable_slicing},
% Equation~\eqref{eq:slicing}:
% \begin{align}
%   \SlicedParameterLayer_c [x,y] = & \sum_{i,j,k} \tent(\GridWidth x-i)\tent(\GridHeight y-j)  \\
%            & \hspace{0.25in} \tent(\GridDepth \Guide [x,y]-k) \ParameterLayer_c [i,j,k] \nonumber \\
%   \frac{\partial \Loss }{\partial \Guide [x,y]} =& \frac{\partial \Loss }{\partial \SlicedParameterLayer_c [x,y]}\frac{\partial \SlicedParameterLayer_c [x,y]}{\partial \Guide [x,y]} \\
%   \frac{\partial \SlicedParameterLayer_c [x,y]}{\partial \Guide [x,y]} =&
%   \sum_{i,j,k} \tent(\GridWidth x-i)\tent(\GridHeight x-j) \\
%            & \hspace{0.25in}  \frac{\partial(\tent(\GridDepth \Guide [x,y]-k))}{\partial \Guide [x,y]} \ParameterLayer_c[i,j,k] \nonumber \\
%   \tent(\GridDepth  x-k) =& \max \left( 1- \left| \GridDepth  x - k \right|, 0 \right) \\
%     \frac{\partial \tent(\GridDepth  x-k)}{\partial x} =& -\GridDepth  \operatorname{sign}(\GridDepth  x-k)\mathbbm{1}_{|\GridDepth  x-k| \leq 1}
% \end{align}

\subsection{Splatting as a neural network}
\label{sec:splatting_as_cnn}
